# Supplementary material for: SimpleRecon: 3D Reconstruction Without 3D Convolutions
Source: arXiv:2208.14743 source file (2022-08-31)
Supplement: Supplementary file 1 [file supp_depth.tex]

\newcommand{\turnwidthnew}{0.9\columnwidth}

\centering

\begin{tabular}{@{\hskip 0.5mm}c@{\hskip 0.5mm}c@{\hskip 0.5mm}c@{\hskip 0.5mm}c@{\hskip 0.5mm}c@{\hskip 0.5mm}c@{}}

{{\hspace{5mm}{\scriptsize RGB}}} &
{{\hspace{7mm}{\scriptsize ESTDepth\cite{long2021multi}}}} &
{{\hspace{1mm}{\scriptsize IDNSolver\cite{zhou2021idn}}}} &
{{\hspace{2mm}{\scriptsize DVMVS\cite{duzceker2021deepvideomvs}}}} &
{{\hspace{8mm}{\scriptsize Ours}}} &
{{\hspace{6mm}{\scriptsize GT}}}\\

\multicolumn{6}{c}{\includegraphics[width=\turnwidthnew]{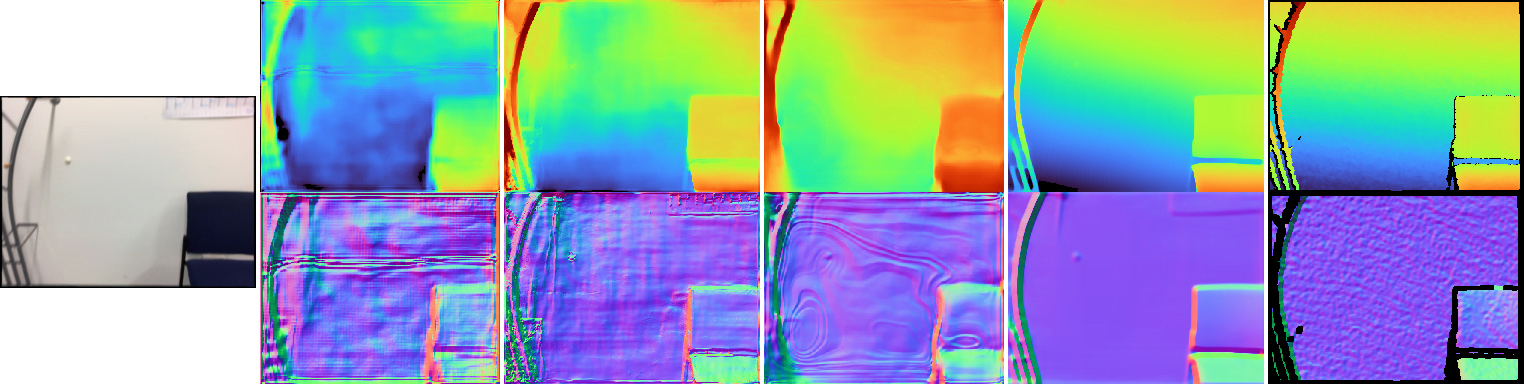}} \\
\multicolumn{6}{c}{\includegraphics[width=\turnwidthnew]{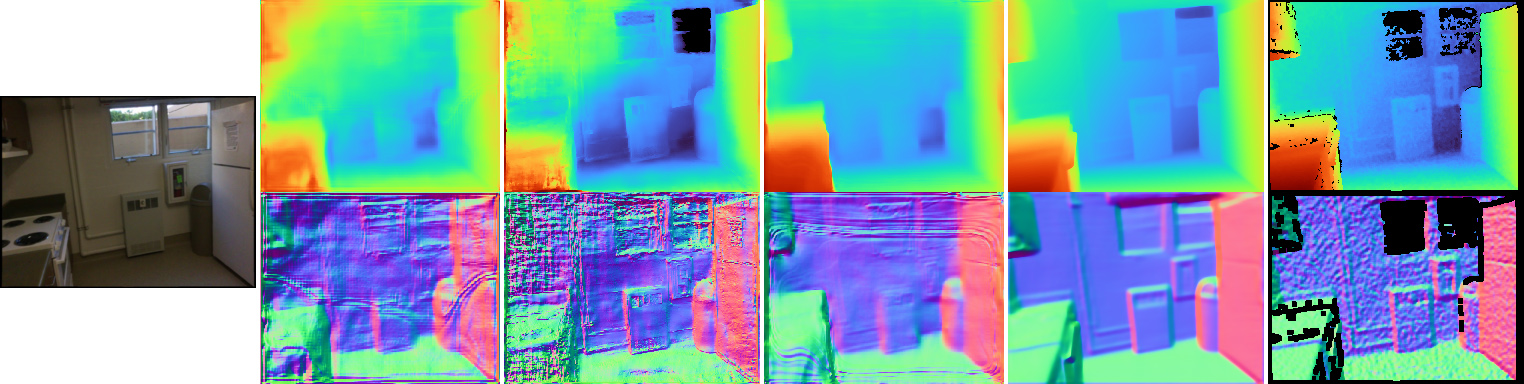}} \\
\multicolumn{6}{c}{\includegraphics[width=\turnwidthnew]{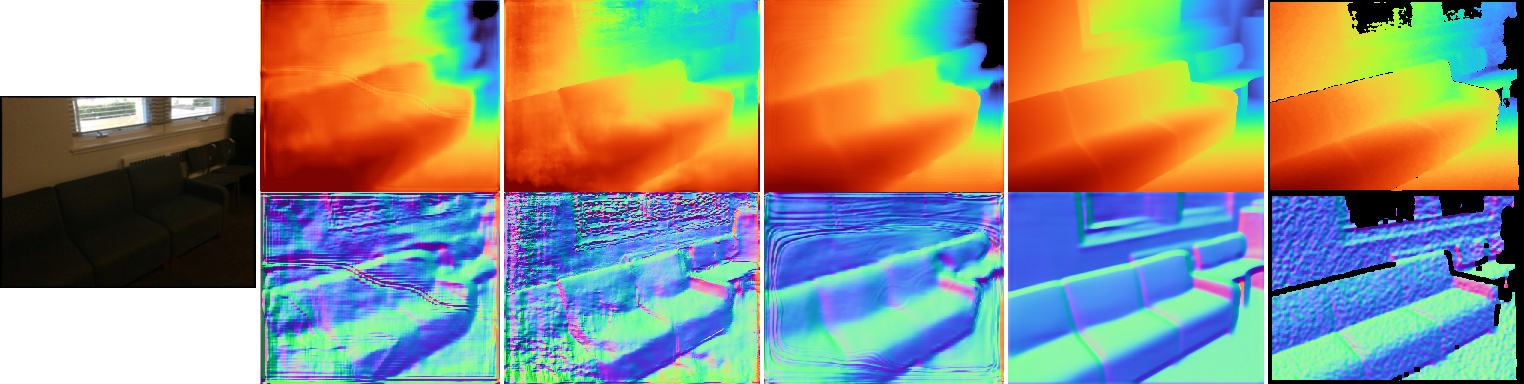}} \\
\multicolumn{6}{c}{\includegraphics[width=\turnwidthnew]{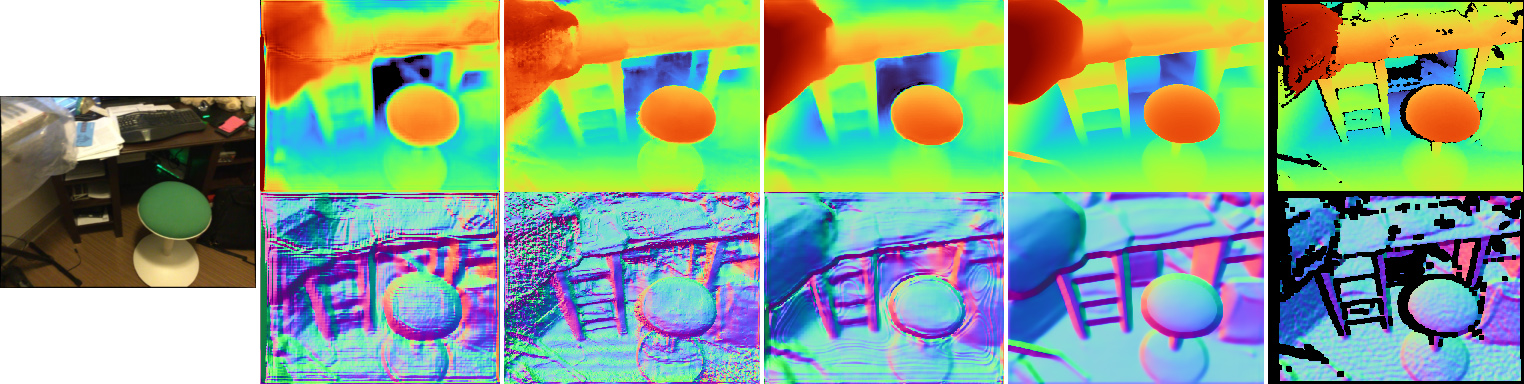}} \\
\multicolumn{6}{c}{\includegraphics[width=\turnwidthnew]{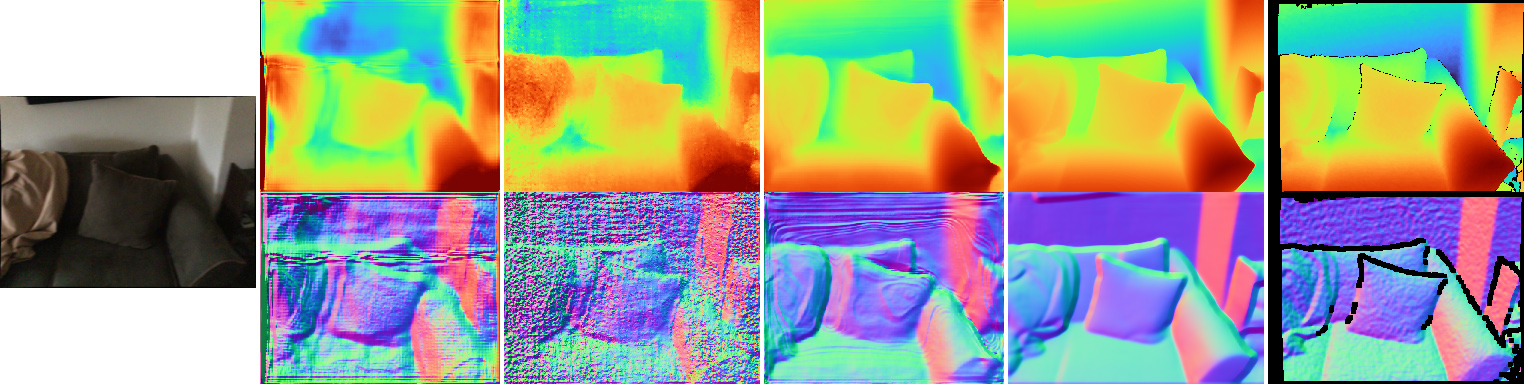}} \\
\multicolumn{6}{c}{\includegraphics[width=\turnwidthnew]{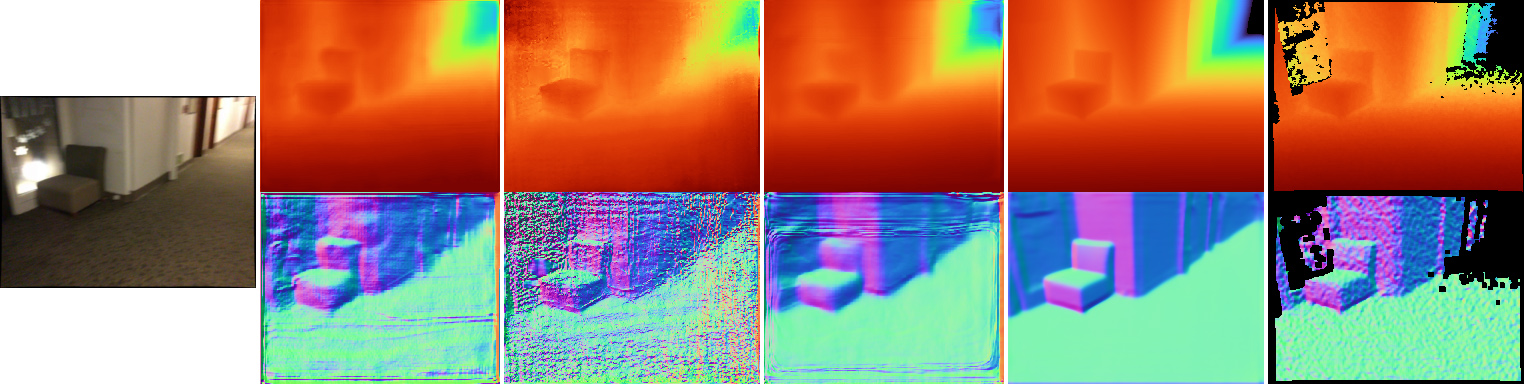}} \\
\end{tabular}
